# Supplementary material for: On the Multi-Reference Nature of Plutonium Oxides: PuO$_2^{2+}$, PuO$_2$, PuO$_3$ and PuO$_2$(OH)$_2$
Source: arXiv:1608.02353 source file (2016-08-08)
Supplement: Supplementary file 1 [file SI.pdf]

# On the Multi-Reference Nature of Plutonium Oxides: $PuO_2^{2+}$, $PuO_2$, $PuO_3$ and $PuO_2(OH)_2$

Katharina Boguslawski,*[a] Florent Réal,[b] Paweł Tecmer,*[a] Corinne Duperrouzel,[b,c] André Severo Pereira Gomes,[b] Örs Legeza,[d] Paul W. Ayers[c], and Valérie Vallet*[b]

[a] *Institute of Physics, Faculty of Physics, Astronomy and Informatics, Nicolaus Copernicus University in Torun, Grudziadzka 5, 87-100 Torun, Poland; E-mail: k.boguslawski@fizyka.umk.pl, ptecmer@fizyka.umk.pl*

[b] *Univ. Lille, CNRS, UMR 8523 - PhLAM - Physique des Lasers Atomes et Molécules, F-59000 Lille, France* [c] *Department of Chemistry and Chemical Biology, McMaster University, Hamilton, 1280 Main Street West, L8S 4M1, Canada*

[d] *Strongly Correlated Systems "Lendület" Research Group, Wigner Research Center for Physics, H-1525 Budapest, Hungary*

## Supporting Information

# 1 XYZ Coordinates in Angstroms

## 1.1 linear $PuO_2$

| | | | |
|---|---|---|---|
| Pu | 0.000000000000 | 0.000000000000 | 0.000000000000 |
| O | 0.000000000000 | 0.000000000000 | 1.814000000000 |
| O | 0.000000000000 | 0.000000000000 | −1.814000000000 |

## 1.2 linear $PuO_2^{2+}$

| | | | |
|---|---|---|---|
| Pu | 0.000000000000 | 0.000000000000 | 0.000000000000 |
| O | 0.000000000000 | 0.000000000000 | 1.711000000000 |
| O | 0.000000000000 | 0.000000000000 | −1.711000000000 |

## 1.3 bent $PuO_2^{2+}$

| | | | |
|---|---|---|---|
| Pu | 0.000000000000 | 0.000000000000 | 0.000000000000 |
| O | −0.118952247373 | 0.000000000000 | 1.762991594661 |
| O | −0.118952247373 | 0.000000000000 | −1.762991594661 |

## 1.4 $PuO_3$

| | | | |
|---|---|---|---|
| Pu | 0.000000000000 | 0.000000000000 | 0.000000000000 |
| O | 1.934000000000 | 0.000000000000 | 0.000000000000 |
| O | −0.118952247373 | 0.000000000000 | 1.762991594661 |
| O | −0.118952247373 | 0.000000000000 | −1.762991594661 |

### 1.5 $PuO_2(OH)_2$

| | | | |
|---|---|---|---|
| Pu | 0.000000000000 | 0.000000000000 | 1.000000000000 |
| O | 1.743451431370 | 0.000000000000 | 0.926500976503 |
| O | −1.743451431370 | 0.000000000000 | 0.926500976503 |
| O | 0.000000000000 | 1.692384295153 | 2.243316290217 |
| O | 0.000000000000 | −1.692384295153 | 2.243316290217 |
| H | 0.779782242822 | 2.098494984571 | 2.631304385035 |
| H | −0.779782242822 | −2.098494984571 | 2.631304385035 |

# 2 DMRG convergence and occupation numbers

Table S1: Ground state energies of all investigated plutonium oxides. The convergence of DMRG calculations with respect to the number of renormalized system states (indicated in brackets) is summarized. The number of block states was kept fixed for $m = 256$ and $m = 512$, while the DBSS procedure was used for larger $m$. [1024]: $m_{\text{min}} = 512$, $m_{\text{init}} = m_{\text{max}} = 1024$, the threshold for the quantum information loss was set to $10^{-5}$. [2048]: $m_{\text{min}} = 512$, $m_{\text{init}} = 1024$, $m_{\text{max}} = 2048$, the threshold for the quantum information loss was set to $10^{-5}$.

| | E/Hartree | | | | |
|---|---|---|---|---|---|
| Molecule | $PuO_2$ | $PuO_2^{2+}$ (linear) | $PuO_2^{2+}$ (bent) | $PuO_3$ | $PuO_2(OH)_2$ |
| DMRG | | | | | |
| FV-CAS | | | | | |
| [256] | – | – | – | – | −852.858 6 |
| [512] | −701.966 0 | −701.224 8 | −701.256 0 | −776.642 0 | −852.862 5 |
| [1024] | −701.967 1 | −701.226 4 | −701.258 8 | −776.642 4 | −852.864 4 |
| [2048] | −701.967 3 | −701.227 1 | −701.260 3 | −776.642 6 | −852.865 5 |
| optCAS | | | | | |
| [256] | – | – | – | −776.611 5 | −852.815 7 |
| [512] | −701.925 8 | −701.202 3 | −701.179 9 | −776.611 5 | −852.816 9 |
| [1024] | −701.925 9 | −701.202 6 | −701.180 2 | – | −852.817 4 |

Table S2: Occupation numbers of each active space orbital with index $i$ for the converged DMRG wavefunctions and investigated plutonium oxides. The orbitals $i$ are ordered as mentioned in the main manuscript.

| $PuO_2$ | | | | $PuO_2^{2+}$ (linear) | | | | $PuO_2^{2+}$ (bent) | | | | $PuO_3$ | | | | $PuO_2(OH)_2$ | | | |
|---|---|---|---|---|---|---|---|---|---|---|---|---|---|---|---|---|---|---|---|
| FV-CAS | | optCAS | | FV-CAS | | optCAS | | FV-CAS | | optCAS | | FV-CAS | | optCAS | | FV-CAS | | optCAS | |
| $i$ | $n_{occ}$ | $i$ | $n_{occ}$ | $i$ | $n_{occ}$ | $i$ | $n_{occ}$ | $i$ | $n_{occ}$ | $i$ | $n_{occ}$ | $i$ | $n_{occ}$ | $i$ | $n_{occ}$ | $i$ | $n_{occ}$ | $i$ | $n_{occ}$ |
| 1 | 2.00 | 1 | 0.02 | 1 | 2.00 | 1 | 1.97 | 1 | 2.00 | 1 | 1.89 | 1 | 2.00 | 1 | 2.00 | 1 | 2.00 | 1 | 1.97 |
| 2 | 2.00 | 2 | 1.99 | 2 | 2.00 | 2 | 0.00 | 2 | 1.99 | 2 | 1.96 | 2 | 2.00 | 2 | 1.98 | 2 | 2.00 | 2 | 1.98 |
| 3 | 1.99 | 3 | 1.98 | 3 | 1.98 | 3 | 1.91 | 3 | 1.99 | 3 | 0.50 | 3 | 2.00 | 3 | 0.24 | 3 | 2.00 | 3 | 2.00 |
| 4 | 0.02 | 4 | 0.99 | 4 | 0.00 | 4 | 0.50 | 4 | 1.89 | 4 | 0.12 | 4 | 2.00 | 4 | 0.00 | 4 | 2.00 | 4 | 1.99 |
| 5 | 0.00 | 5 | 0.07 | 5 | 0.00 | 5 | 0.10 | 5 | 1.95 | 5 | 1.89 | 5 | 1.99 | 5 | 1.98 | 5 | 2.00 | 5 | 0.47 |
| 6 | 0.00 | 6 | 1.99 | 6 | 0.00 | 6 | 1.91 | 6 | 0.50 | 6 | 0.12 | 6 | 2.00 | 6 | 1.99 | 6 | 1.99 | 6 | 0.54 |
| 7 | 1.99 | 7 | 1.98 | 7 | 1.99 | 7 | 0.50 | 7 | 0.13 | 7 | 0.50 | 7 | 1.98 | 7 | 0.78 | 7 | 1.97 | 7 | 0.00 |
| 8 | 1.98 | 8 | 0.99 | 8 | 1.91 | 8 | 0.10 | 8 | 0.01 | 8 | 1.90 | 8 | 0.22 | 8 | 0.00 | 8 | 1.98 | 8 | 0.00 |
| 9 | 0.99 | 9 | 0.07 | 9 | 0.49 | 9 | 1.92 | 9 | 0.01 | 9 | 1.96 | 9 | 0.00 | 9 | 0.02 | 9 | 1.99 | 9 | 0.02 |
| 10 | 0.07 | 10 | 1.93 | 10 | 0.10 | 10 | 0.51 | 10 | 0.00 | 10 | 0.51 | 10 | 0.01 | 10 | 1.98 | 10 | 1.99 | 10 | 0.02 |
| 11 | 1.99 | 11 | 0.95 | 11 | 1.99 | 11 | 0.09 | 11 | 1.99 | 11 | 0.13 | 11 | 0.01 | 11 | 1.97 | 11 | 0.47 | 11 | 1.97 |
| 12 | 1.98 | 12 | 0.07 | 12 | 1.91 | 12 | 1.96 | 12 | 1.89 | 12 | 0.03 | 12 | 1.99 | 12 | 0.26 | 12 | 0.55 | 12 | 1.98 |
| 13 | 0.99 | 13 | 1.99 | 13 | 0.52 | 13 | 0.03 | 13 | 0.50 | 13 | 1.95 | 13 | 1.98 | 13 | 0.01 | 13 | 0.01 | 13 | 1.97 |
| 14 | 0.07 | 14 | 0.02 | 14 | 0.10 | 14 | 1.96 | 14 | 0.13 | 14 | 0.51 | 14 | 1.99 | 14 | 0.78 | 14 | 0.00 | 14 | 2.00 |
| 15 | 0.01 | 15 | 1.99 | 15 | 0.01 | 15 | 0.03 | 15 | 0.01 | 15 | 0.03 | 15 | 0.81 | | | 15 | 0.03 | 15 | 2.00 |
| 16 | 2.00 | 16 | 0.02 | 16 | 1.99 | 16 | 0.51 | 16 | 0.00 | | | 16 | 0.01 | | | 16 | 0.03 | 16 | 0.56 |
| 17 | 1.99 | 17 | 0.96 | 17 | 1.99 | | | 17 | 1.99 | | | 17 | 0.03 | | | 17 | 0.00 | 17 | 0.45 |
| 18 | 1.93 | | | 18 | 1.91 | | | 18 | 1.99 | | | 18 | 2.00 | | | 18 | 0.00 | 18 | 0.00 |
| 19 | 0.96 | | | 19 | 0.50 | | | 19 | 1.89 | | | 19 | 2.00 | | | 19 | 2.00 | 19 | 0.01 |
| 20 | 0.07 | | | 20 | 0.08 | | | 20 | 1.95 | | | 20 | 1.99 | | | 20 | 2.00 | 20 | 0.01 |
| 21 | 1.99 | | | 21 | 1.96 | | | 21 | 0.51 | | | 21 | 1.97 | | | 21 | 2.00 | 21 | 0.02 |
| 22 | 0.02 | | | 22 | 0.03 | | | 22 | 0.13 | | | 22 | 1.96 | | | 22 | 1.99 | 22 | 0.04 |
| 23 | 1.99 | | | 23 | 1.96 | | | 23 | 0.04 | | | 23 | 0.25 | | | 23 | 1.99 | | |
| 24 | 0.02 | | | 24 | 0.03 | | | 24 | 1.95 | | | 24 | 0.01 | | | 24 | 1.96 | | |
| 25 | 0.96 | | | 25 | 0.52 | | | 25 | 0.51 | | | 25 | 2.00 | | | 25 | 1.97 | | |
| | | | | | | | | 26 | 0.04 | | | 26 | 0.81 | | | 26 | 1.96 | | |
| | | | | | | | | | | | | | | | | 27 | 1.99 | | |
| | | | | | | | | | | | | | | | | 28 | 1.99 | | |
| | | | | | | | | | | | | | | | | 29 | 0.58 | | |
| | | | | | | | | | | | | | | | | 30 | 0.44 | | |
| | | | | | | | | | | | | | | | | 31 | 0.00 | | |
| | | | | | | | | | | | | | | | | 32 | 0.02 | | |
| | | | | | | | | | | | | | | | | 33 | 0.01 | | |
| | | | | | | | | | | | | | | | | 34 | 0.03 | | |
| | | | | | | | | | | | | | | | | 35 | 0.05 | | |
